# Supplementary material for: Strong-field electro-optic sampling of light
Source: arXiv:2410.19196 source file (2026-09-20)
Supplement: Supplementary file 1 [file SI.tex]

\documentclass[pdflatex,sn-mathphys-num]{sn-jnl}% Math and Physical Sciences Numbered Reference Style 
%%\documentclass[pdflatex,sn-mathphys-ay]{sn-jnl}% Math and Physical Sciences Author Year Reference Style
%%\documentclass[pdflatex,sn-aps]{sn-jnl}% American Physical Society (APS) Reference Style
%%\documentclass[pdflatex,sn-vancouver,Numbered]{sn-jnl}% Vancouver Reference Style
%%\documentclass[pdflatex,sn-apa]{sn-jnl}% APA Reference Style 
%%\documentclass[pdflatex,sn-chicago]{sn-jnl}% Chicago-based Humanities Reference Style

%%%% Standard Packages
%%<additional latex packages if required can be included here>

\usepackage{graphicx}%
\usepackage{multirow}%
\usepackage{amsmath,amssymb,amsfonts}%
\usepackage{amsthm}%
\usepackage{mathrsfs}%
\usepackage[title]{appendix}%
\usepackage{xcolor}%
\usepackage{textcomp}%
\usepackage{manyfoot}%
\usepackage{booktabs}%
\usepackage{algorithm}%
\usepackage{algorithmicx}%
\usepackage{algpseudocode}%
\usepackage{listings}%
\usepackage[LGRgreek]{mathastext}%
%%%%

%%%%%=============================================================================%%%%
%%%%  Remarks: This template is provided to aid authors with the preparation
%%%%  of original research articles intended for submission to journals published 
%%%%  by Springer Nature. The guidance has been prepared in partnership with 
%%%%  production teams to conform to Springer Nature technical requirements. 
%%%%  Editorial and presentation requirements differ among journal portfolios and 
%%%%  research disciplines. You may find sections in this template are irrelevant 
%%%%  to your work and are empowered to omit any such section if allowed by the 
%%%%  journal you intend to submit to. The submission guidelines and policies 
%%%%  of the journal take precedence. A detailed User Manual is available in the 
%%%%  template package for technical guidance.
%%%%%=============================================================================%%%%

%% as per the requirement new theorem styles can be included as shown below
\theoremstyle{thmstyleone}%
%  meant for continuous numbers
%%\newtheorem{theorem}{Theorem}[section]% meant for sectionwise numbers
%% optional argument [theorem] produces theorem numbering sequence instead of independent numbers for Proposition
% 
%%\newtheorem{proposition}{Proposition}% to get separate numbers for theorem and proposition etc.

\theoremstyle{thmstyletwo}%

\theoremstyle{thmstylethree}%

\raggedbottom
%%\unnumbered% uncomment this for unnumbered level heads

\begin{document}

\title[Article Title]{Supplementary materials for towards multi-petahertz all-optical electric field sampling}

%%=============================================================%%
%% GivenName	-> \fnm{Joergen W.}
%% Particle	-> \spfx{van der} -> surname prefix
%% FamilyName	-> \sur{Ploeg}
%% Suffix	-> \sfx{IV}
%% \author*[1,2]{\fnm{Joergen W.} \spfx{van der} \sur{Ploeg} 
%%  \sfx{IV}}\email{iauthor@gmail.com}
%%=============================================================%%

\author[1]{\fnm{Anton} \sur{Husakou}}

\author[2,3]{\fnm{Nicholas} \sur{Karpowicz}}

\author[2,3]{\fnm{Vladislav S.} \sur{Yakovlev}}

\author[1]{\fnm{Misha} \sur{Ivanov}}

\author[4]{\fnm{Dmitry A.} \sur{Zimin}}

\affil[1]{\orgname{Max Born Institute for Nonlinear Optics and Short Pulse Spectroscopy}, \orgaddress{\city{Berlin}, \country{Germany}}}

\affil[2]{\orgname{Max-Planck-Institut f\"ur Quantenoptik}, \orgaddress{\city{Garching}, \country{Germany}}}

\affil[3]{\orgdiv{Fakult\"at für Physik}, \orgname{Ludwig-Maximilians-Universit\"at}, \orgaddress{\city{Garching}, \country{Germany}}}

\affil[4]{\orgdiv{Laboratory of Physical Chemistry}, \orgname{ETH
Zurich}, \orgaddress{\city{Z\"urich}, \country{Switzerland}}}

\maketitle

\section{Evolution of the Green function}

The Green function is a function of the propagation coordinate and is explicitly denoted by $G(z,t,\tau')$. Its propagation equation is given by

\begin{equation}
    \frac{\partial G(z,\omega_0,\omega)}{\partial z}=i\beta(\omega_0)G(z,\omega_0,\omega)+P(z,\omega_0),
\end{equation} \\
where 

\begin{equation}
    P(z,t)=\alpha(z,t)G(z,t,\tau')+\frac{[\partial \beta(z,t)G(z,t,\tau')]}{\partial t}+\int_{-\infty}^t\gamma(z,\tau'')G(z,\tau'',\tau')d\tau''
\end{equation}

Note that the propagation equation for the Green function is linear, reflecting the fact that the signal field is considered small. Finally, the expressions for the functions $\alpha(z,t)$ and $\beta(z,t)$ are given in terms of the sampling field $E_S(z,t)$ and the induced relative plasma density $\rho(z,t)$:

\begin{equation}
    \alpha(z,t)=-\frac{N_0I_p}{2c\epsilon_0E_S^2(z,t)}\frac{\partial \rho(z,t)}{\partial t},
\end{equation}

\begin{equation}
    \beta(z,t)=-\frac{\chi_3}{2c}E_S^2(z,t),
\end{equation}

\begin{equation}
    \gamma(z,t)=-\frac{N_0e^2}{2c\epsilon_0m_e}\rho(z,t).
\end{equation} \\

Here, $N_0$ is the concentration of atoms/molecules, $I_p$ is the bandgap, $c$ is the vacuum light velocity, $\epsilon_0$ is the vacuum permittivity, $\chi_3$ is the third-order susceptibility which describes the mixing of two photons of the pump field and, one photon of the signal, $m_e$ is the (effective) electron mass.

\section{Distribution of plasma density with the propagation length}

\begin{figure}[!ht]
\center{\includegraphics[width=0.45\textwidth]{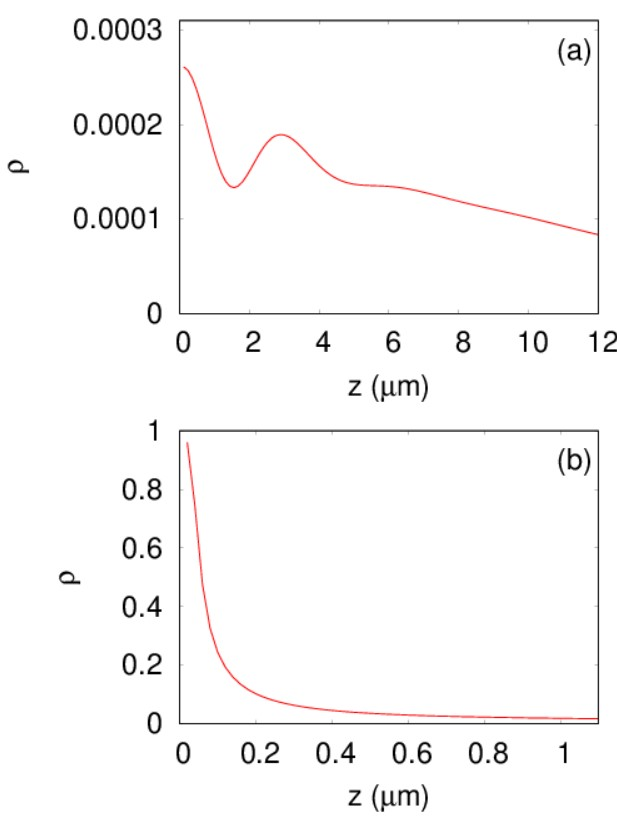}}
\caption{\label{plasma}Dependence of the plasma density $\rho$ after the sampling pulse on the propagation coordinate, for the sampling pulse field strength of 1.54 V/\AA (a) and 5 V/\AA (b).}
\end{figure}

In Fig. \ref{plasma}, we show the distribution of the plasma in the sample, according to the simulations. One can see that even for the field of 1.54 V/\AA, we predict that plasma is concentrated near the front surface of the sample. The reason for this is sampling pulse absorption due to photoionization (pump depletion). The concentration of carriers near the front surface becomes even more pronounced for higher intensities of the sampling pulse, as shown in Fig. \ref{plasma}(b). Therefore for high intensities, plasma-related processes are concentrated in the very thin layer at the entrance surface, indicating that it would be useful to consider a very thin free-standing film as a nonlinear medium.

\section{Separation of the IS and DS terms in the nonlinear response}
To separate IS and DS terms, we formally split the real-valued electric field $E(t)$ into positive-frequency and negative-frequency complex-valued time-dependent components as

\begin{equation}
E^\pm(t)=\hat{F}^{-1}\{[0.5\pm0.5H(\omega)]\hat{F}[E(t)]\},
\end{equation} \\
where $\hat{F}$ is the Fourier transform and $\hat{F}^{-1}$ is its inversion, while $H(\omega)$ is the Heaviside function.
After some straightforward algebraic manipulations, we show that the corresponding terms in the polarization $P_{NL}(t)=P_{NL,IS}(t)+P_{NL,DS}(t)$ look like 

\begin{equation}
  P_{NL,IS}(t)=0.75\epsilon_0\chi_3E(t)^3+0.75\epsilon_0\chi_3C(t)^3  
\end{equation}
and 

\begin{equation}
   P_{NL,DS}(t)=0.25\epsilon_0\chi_3E(t)^3-0.75\epsilon_0\chi_3C(t)^3,
\end{equation} \\
where we define an auxiliary real-valued electric field $C(t)=\hat{F}^{-1}\{[-1+2H(\omega)]\hat{F}[E(t)]\}$.

\section{Optical system}
\label{laser_beamline}

\begin{figure}[ht!]
\centering
	\includegraphics[scale=0.6]{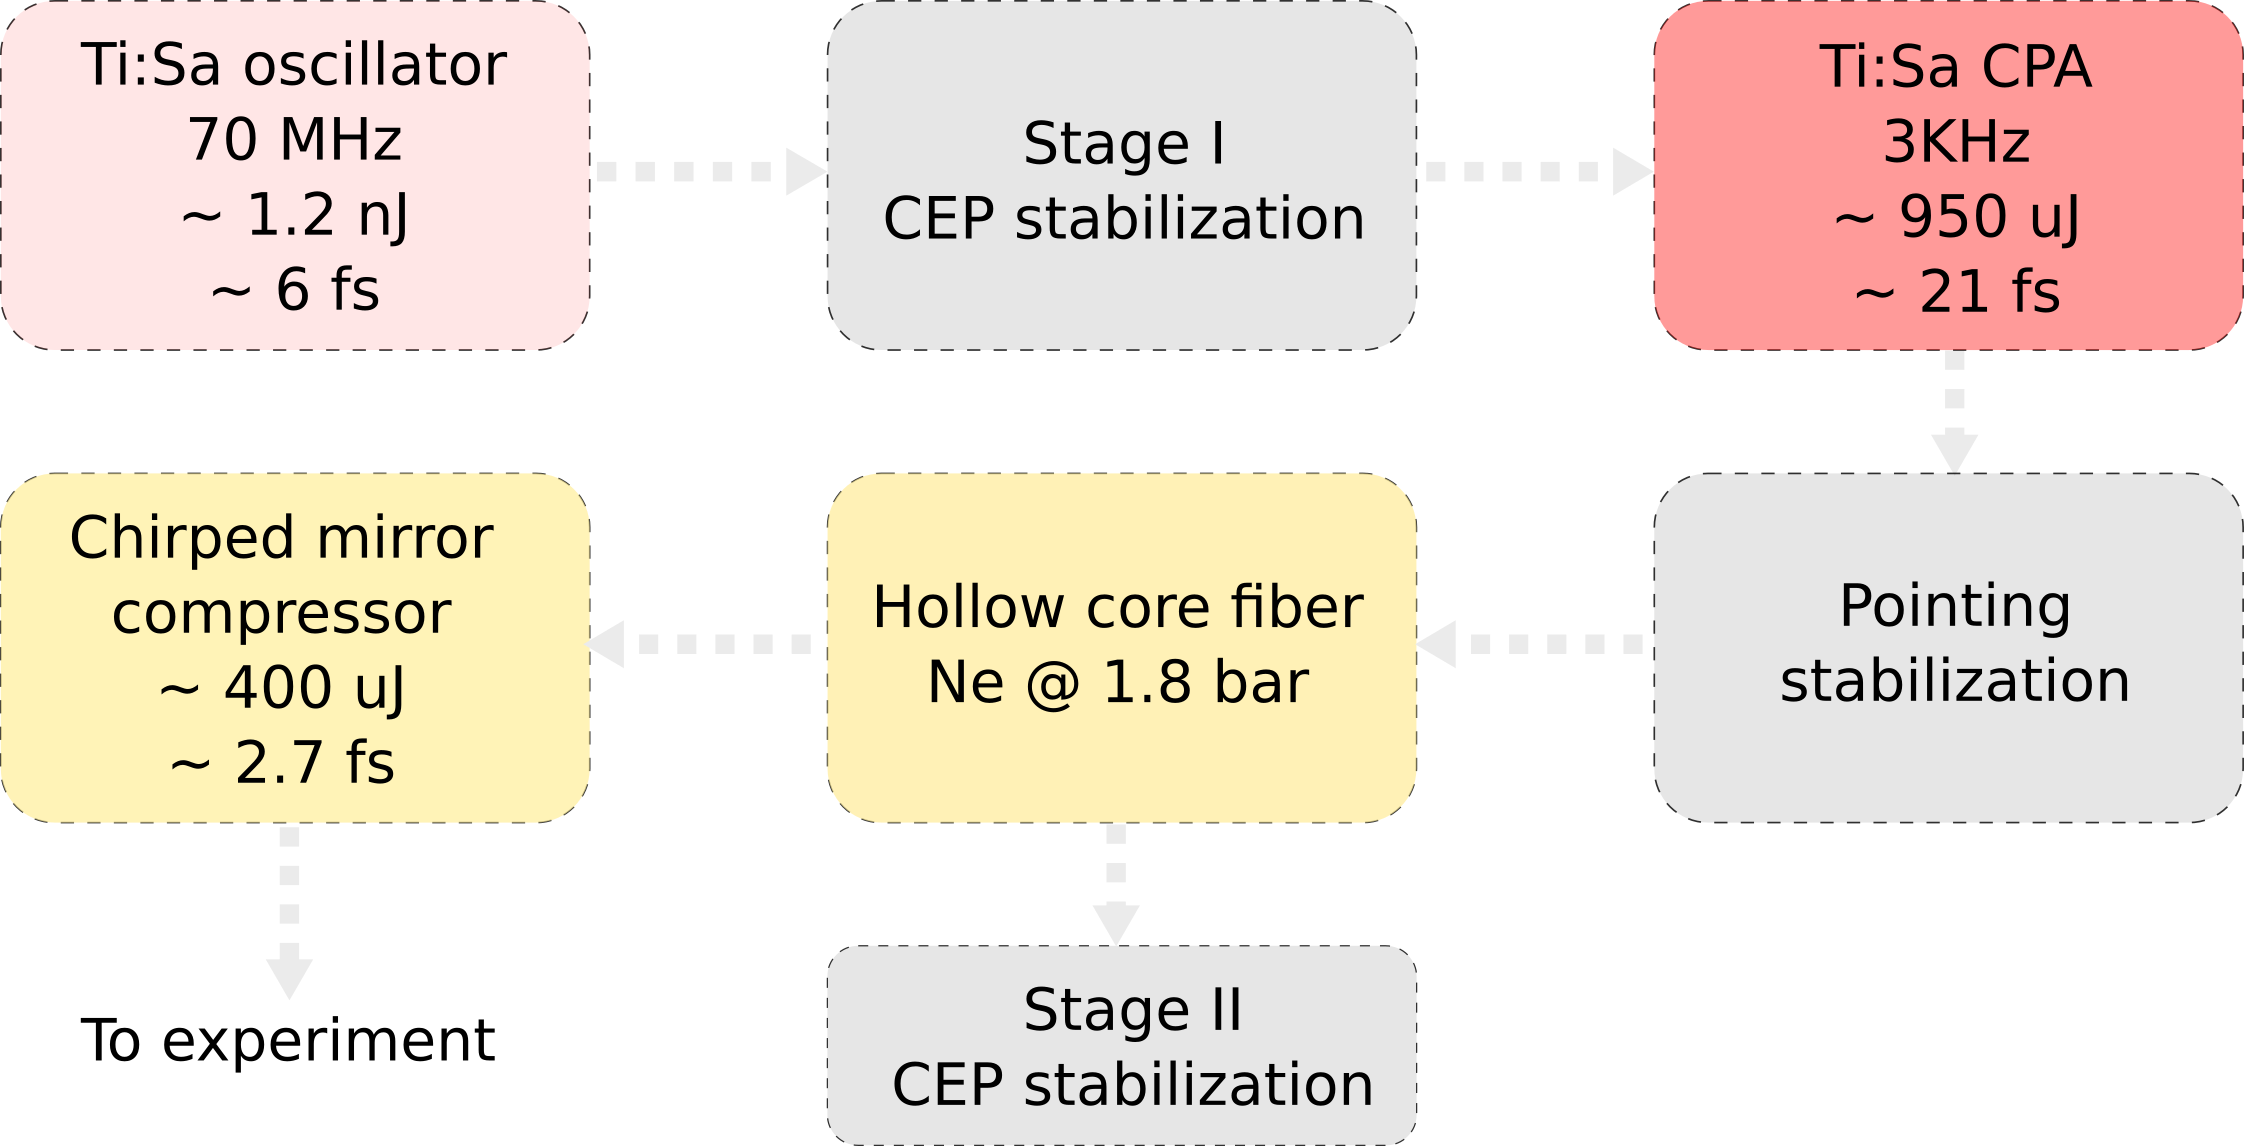}
	\caption{Diagram of the experimental beam-line.}
	\label{fp2_scheme}
\end{figure}

Fig.~\ref{fp2_scheme} shows a schematic of the laser beamline\cite{Cavalieri_2007, Tim_thesis} used for the experiments.
Ti:sapphire oscillator (Rainbow 2, Spectra Physics) provides an octave-spanning bandwidth with about $\sim 750$~nm central wavelength.
The output from the oscillator is guided through the "stage I" CEP stabilization module based on the feed-forward scheme\cite{Tim_thesis}.
CEP stable pulses are further amplified within a 9-pass cryo-cooled Ti:sapphire chirped-pulse amplifier at a repetition rate of 3~kHz, and temporally compressed using a transmission grating-based compressor yielding $\sim 21$~fs pulses with $\sim 2.5$~W output power.
The amplified pulses are further spectrally broadened in a hollow-core fiber (HCF), filled with 1.8 bar of neon gas resulting in a spectral broadening to a bandwidth of about 450 - 1000 nm.
The chirped mirror compressor consisting of 3 pairs of chirped mirrors in combination with about 6~mm of fused silica glass and 50~cm of air is then used to compress the broadened spectrum to about $\sim 2.7$~fs (FWHM) duration pulse\cite{Sederberg2020}. The compressed pulses are guided to the experimental setup. The small fraction of spectrally broadened light is reflected from the Brewster window of the hollow core fiber sealing and guided to a 'Stage II CEP stabilization'. The Stage II stabilization is based on f-to-2f technique~\cite{schultze_thesis}.

\section{Data acquisition}
\label{acquisition}

The signal from GHOST detection was a current generated by a photodiode (ALPHALAS). This current was first converted into voltage with further amplification by a transimpedance amplifier (DLPCA-200, FEMTO Messtechnik).
The amplified voltage signal was connected to a dual-phase lock-in amplifier (SR-830, Stanford Research Systems), triggered by an electrical signal synchronized with half of the repetition rate of the laser.

The measured signal from the lock-in amplifier was read by software on a computer via GPIB interface (National Instruments).

\section{Sample medium characterization}
\label{thickness_section}

In order to precisely determine the spectral response, the propagation effects within a nonlinear medium should be considered. For this, the precise thickness of the medium must be known. The thickness can be determined with a conventional spectrometer and a broadband light source. An optical pulse gets reflected at both surfaces of a sample. After an even number of reflections, light travels in the same direction as the incident pulse, but it is delayed due to a longer propagation through the medium. Multiple pulses in the time domain will result in spectral fringes, which can be measured with a spectrometer. The total transmission of a medium, which takes into account reflections at the surfaces, is given by
\begin{equation}
T(n,\omega, d) = \frac{1}{\cos \left( \frac{\omega}{c}n d \right) - \frac{i}{2} \left( n + \frac{1}{n} \right) \sin \left( \frac{\omega}{c} n d \right)},
\label{thickness_equation}
\end{equation} \\
where $T$ is the intensity transmission, $n$ is the real-valued refractive index at a frequency $\omega$, $c$ is the vacuum speed of light, and $d$ is the sample thickness.

To precisely measure the thickness of $z$-cut $\alpha$-quartz sample, the intensity spectrum of a broadband pulse (section \ref{laser_beamline}) was measured with and without the sample (Fig.~\ref{thickness_measurement}).
The spacing of fringes was then modeled with Eq.~\eqref{thickness_equation}, where we evaluated the frequency-dependent refractive index using the Sellmeier equation\cite{Ghosh1999}.
The calculated sample thickness is the one that provides the best agreement of fringe positions in the experiment.

\begin{figure}[ht!]
\centering
	\includegraphics[scale=0.25]{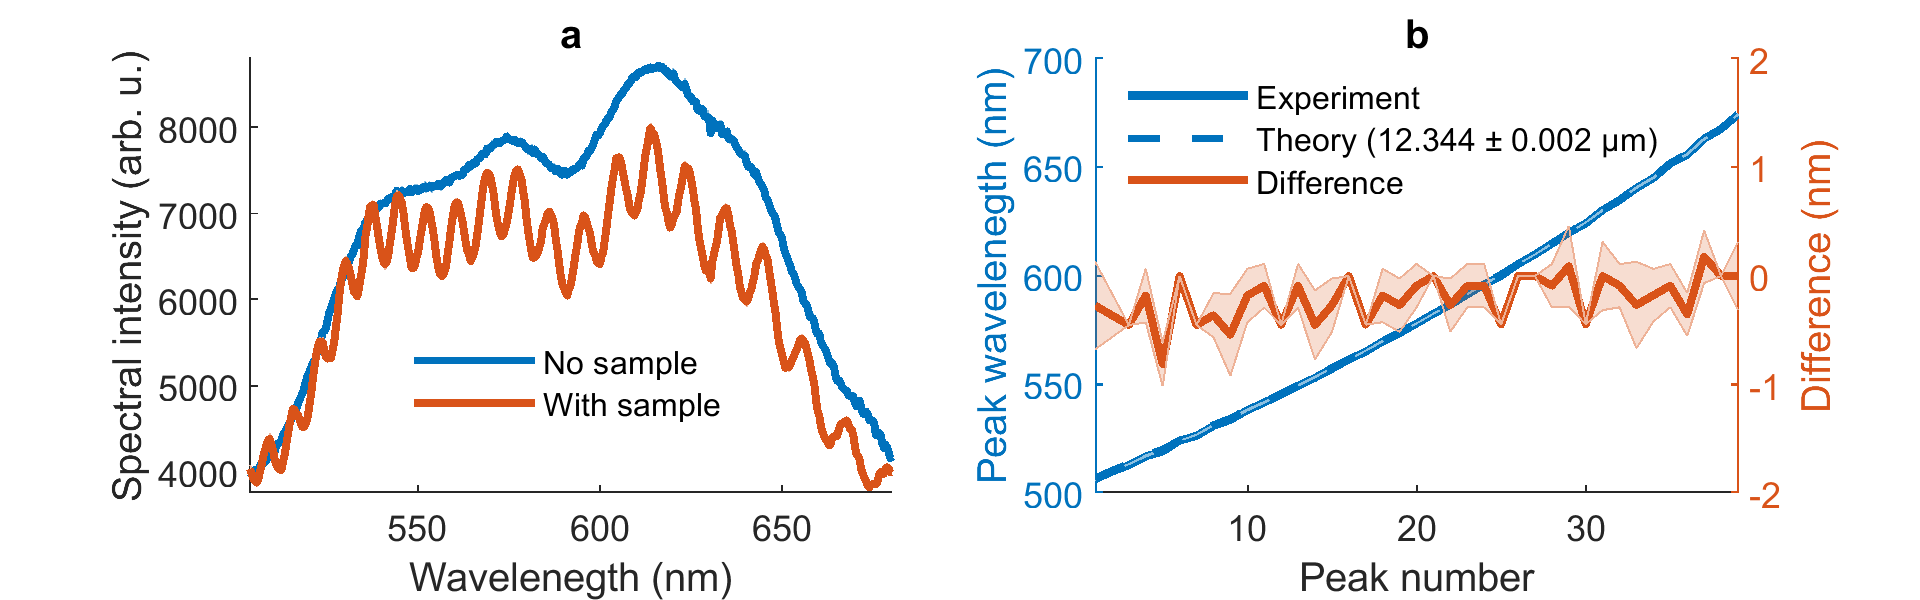}
	\caption{Measured change of spectral intensities  with a $z$-cut $\alpha$-quartz sample (\textbf{a}).
	Positions of spectral fringes allow extracting a sample thickness for the sample (\textbf{b}).}
	\label{thickness_measurement}
\end{figure}

The $z$-cut $\alpha$-quartz crystal sample was provided by MTI Corporation, and its thickness was further reduced by polishing.

\section{Experimental setup}
\label{schematics}

\begin{figure}[ht!]
\centering
	\includegraphics[scale=0.8]{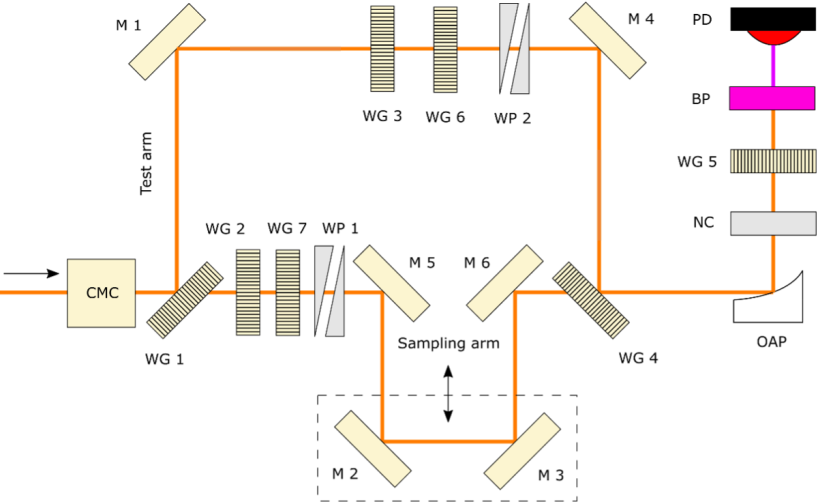}
	\caption{Optical setup. WG – wire-grid polarizer, WP – wedge pair, M – protected silver mirror, NC – nonlinear crystal, BP – bandpass filter, PD – photodiode, CMC – chirped mirror compressor. }
	\label{ghost_visible}
\end{figure}

The experimental setup is shown in Fig. \ref{ghost_visible}. After the chirped mirror compressor (CMC), the pulse is split into two optical arms (sampling and test). The test pulse is transmitted through the set of wire-gird polarizers (WG 3, WG 6) for adjusting the pulse energy. The wedge pair (WP 2) is used for the fine-tuning the compression of the test pulse. After setting the test pulse energy and compression, the pulse is recombined with the sampling arm by the wire-grid polarizer WG 4.

The sampling pulse undergoes a similar procedure as the test pulse where the wire-grid polarizers WG 2 and WG 7 are used to set the pulse energy while the wedge pair WP 1 is used for fine-tuning the pulse compression. The delay line consisting of M 2 and M 3 protected silver mirrors placed on a linear closed-loop piezo stage (PX 200, Piezosystems Jena) for adjusting the delay between sampling and test pulses. 

After recombination of the sampling and test pulses with the wire grid, both cross-polarized pulses are focused with an off-axis protected silver parabolic mirror (OAP) on the nonlinear crystal (NC). The nonlinear crystal is a z-cut $\alpha$-quartz crystal of ~ 12 $\mu$m thickness. The emerging local oscillator and a signal are chosen \cite{ghost} by means of the wire-grid polarizer WG 5, while the detection frequency is defined by the narrow bandpass filter centred at about 0.845 PHz. The interfering local oscillator and the signal are incident on a photodiode.

\section{The spectral response of the photodiode and bandpass filter}

To get a more accurate experimental spectral response of detection, as well as to perform simulations close to experimental conditions, we took into account the spectral sensitivity of the photodiode (ALPHALAS GmBH) and the transmission of the bandpass filter (Thorlabs) (Fig.~\ref{diode_response}).
 ALPHALAS GmBH provided the spectral sensitivity of the photodiode.

\begin{figure}[ht!]
\centering
	\includegraphics[scale=0.25]{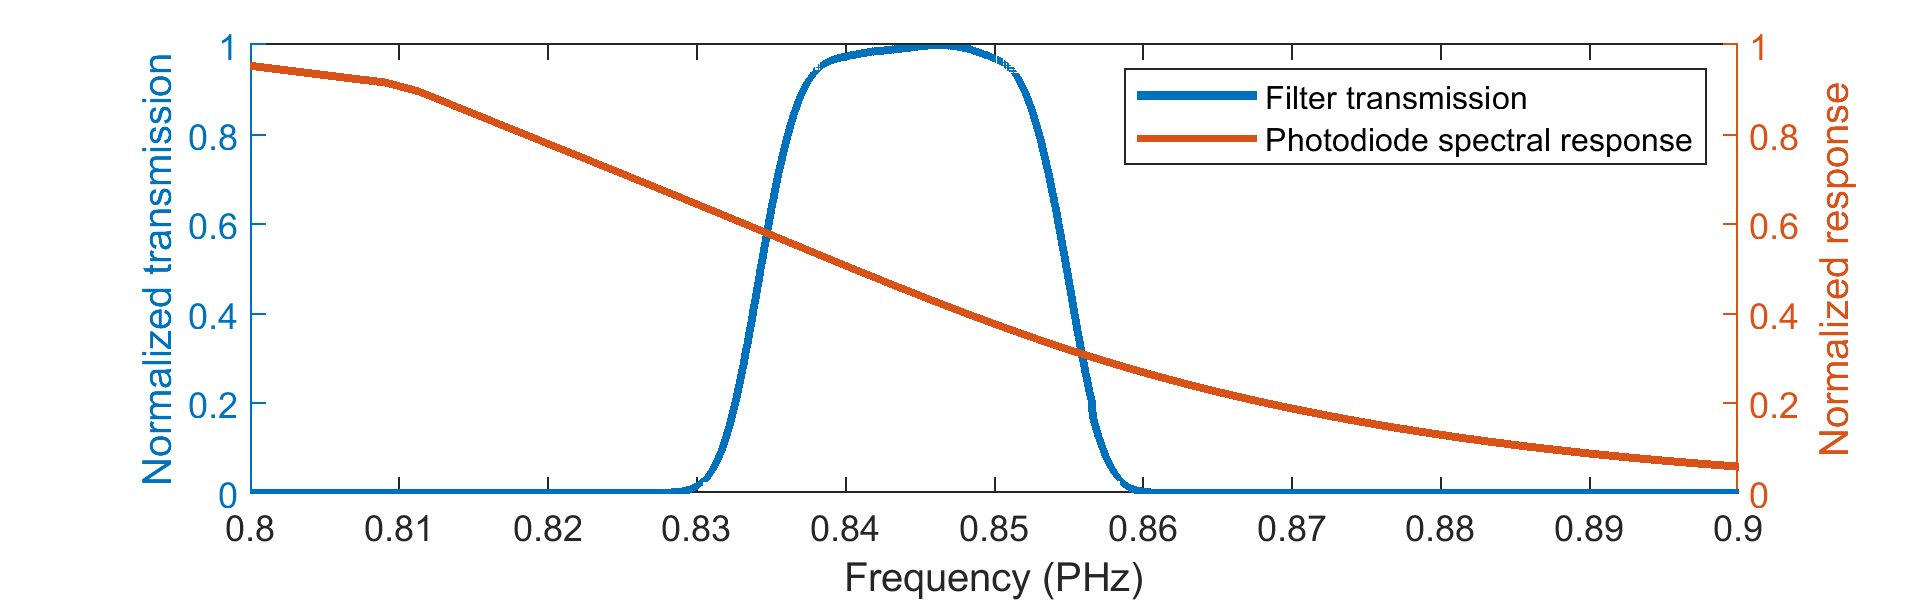}
	\caption{The spectral response of the photo-diode and the measured transmission of the bandpass filter used in the experiment.}
	\label{diode_response}
\end{figure}

\end{document}
